# Supplementary material for: The DeepSpeak Dataset
Source: arXiv:2408.05366 source file (2026-04-06)
Supplement: Supplementary file 1 [file video_identity_pairs.tex]

\begin{table}[!h]
\centering

\caption{Video identity pairs found through the minimal cosine distance between mean CLIP embeddings of five video frames.} %  Part 1/2.
%\vspace{0.5cm}
\resizebox{0.89\textwidth}{!}{
\begin{minipage}{0.32\linewidth}
\centering
\begin{tabular}{|l|l|}
\hline
identity\_1 & identity\_2 \\ \hline
0 & 1 \\
2 & 3 \\
4 & 5 \\
6 & 7 \\
8 & 9 \\
10 & 11 \\
12 & 13 \\
14 & 15 \\
16 & 17 \\
18 & 19 \\
20 & 21 \\
22 & 23 \\
24 & 25 \\
26 & 27 \\
28 & 29 \\
30 & 31 \\
32 & 33 \\
34 & 35 \\
37 & 38 \\
39 & 40 \\
41 & 42 \\
43 & 44 \\
45 & 46 \\
47 & 48 \\
49 & 50 \\
51 & 52 \\
53 & 54 \\
55 & 56 \\
57 & 58 \\
59 & 60 \\
61 & 62 \\
63 & 64 \\
65 & 66 \\
67 & 68 \\
69 & 70 \\
71 & 72 \\
73 & 74 \\
75 & 76 \\
77 & 78 \\
79 & 80 \\
81 & 82 \\
83 & 84 \\
\hline
\end{tabular}
\end{minipage}
\hfill
\begin{minipage}{0.32\linewidth}
\centering
\begin{tabular}{|l|l|}
\hline
identity\_1 & identity\_2 \\ \hline
85 & 86 \\
87 & 192 \\
88 & 126 \\
89 & 106 \\
90 & 194 \\
91 & 119 \\
92 & 184 \\
93 & 207 \\
94 & 191 \\
95 & 201 \\
96 & 142 \\
97 & 98 \\
99 & 100 \\
101 & 174 \\
102 & 196 \\
103 & 134 \\
104 & 193 \\
105 & 177 \\
107 & 170 \\
108 & 109 \\
110 & 111 \\
112 & 113 \\
114 & 115 \\
116 & 124 \\
117 & 208 \\
118 & 165 \\
120 & 129 \\
121 & 214 \\
122 & 137 \\
123 & 162 \\
125 & 220 \\
127 & 172 \\
128 & 164 \\
130 & 152 \\
131 & 149 \\
132 & 206 \\
133 & 173 \\
135 & 205 \\
136 & 219 \\
138 & 145 \\
139 & 185 \\
140 & 141 \\
\hline
\end{tabular}
\end{minipage}
\hfill
\begin{minipage}{0.32\linewidth}
\centering
\begin{tabular}{|l|l|}
\hline
identity\_1 & identity\_2 \\ \hline
143 & 144 \\
146 & 171 \\
147 & 154 \\
148 & 155 \\
150 & 151 \\
153 & 163 \\
156 & 157 \\
158 & 159 \\
160 & 161 \\
166 & 167 \\
168 & 178 \\
169 & 202 \\
175 & 198 \\
176 & 197 \\
179 & 218 \\
180 & 181 \\
182 & 183 \\
186 & 215 \\
187 & 217 \\
188 & 211 \\
189 & 190 \\
195 & 221 \\
199 & 200 \\
203 & 204 \\
209 & 210 \\
212 & 213 \\
222 & 258 \\
223 & 419 \\
224 & 230 \\
225 & 411 \\
226 & 270 \\
227 & 400 \\
228 & 480 \\
229 & 253 \\
231 & 414 \\
232 & 361 \\
233 & 462 \\
234 & 264 \\
235 & 393 \\
236 & 467 \\
237 & 383 \\
~ & ~ \\
\hline
\end{tabular}
\end{minipage}
}
\label{tab:identity_pairs_1}
\end{table}
