# Supplementary material for: The DeepSpeak Dataset
Source: arXiv:2408.05366 source file (2026-04-06)
Supplement: Supplementary file 2 [file audio_identity_pairs.tex]

\begin{table}[!ht]
\centering
\caption{Audio identity pairs generated by taking the minimal cosine distance between vectors comprising 192-dimensional TitaNet embedding values.}
\vspace{0.5cm}
\begin{minipage}{0.32\linewidth}
\centering
\begin{tabular}{|l|l|}
\hline
identity\_1 & identity\_2 \\ \hline
152 & 491 \\ 
10 & 32 \\ 
393 & 404 \\ 
43 & 285 \\ 
236 & 333 \\ 
364 & 371 \\ 
135 & 255 \\ 
130 & 455 \\ 
151 & 268 \\ 
105 & 466 \\ 
120 & 374 \\ 
132 & 294 \\ 
74 & 362 \\ 
103 & 112 \\ 
18 & 219 \\ 
147 & 467 \\ 
162 & 192 \\ 
109 & 332 \\ 
157 & 405 \\ 
241 & 437 \\ 
% Continue as needed...
\hline
\end{tabular}
\end{minipage}
\hfill
\begin{minipage}{0.32\linewidth}
\centering
\begin{tabular}{|l|l|}
\hline
identity\_1 & identity\_2 \\ \hline
104 & 180 \\
35 & 174 \\
53 & 445 \\
70 & 377 \\
51 & 244 \\
281 & 501 \\
44 & 189 \\
270 & 359 \\
357 & 413 \\
69 & 273 \\
209 & 350 \\
200 & 277 \\
345 & 366 \\
65 & 478 \\
11 & 344 \\
62 & 66 \\
153 & 399 \\
54 & 226 \\
129 & 278 \\
95 & 114 \\
% Continue as needed...
\hline
\end{tabular}
\end{minipage}
\hfill
\begin{minipage}{0.32\linewidth}
\centering
\begin{tabular}{|l|l|}
\hline
identity\_1 & identity\_2 \\ \hline
52 & 386 \\
90 & 227 \\
170 & 410 \\
19 & 265 \\
4 & 338 \\
203 & 476 \\
186 & 261 \\
56 & 86 \\
61 & 312 \\
206 & 330 \\
111 & 428 \\
41 & 214 \\
423 & 482 \\
418 & 459 \\
88 & 149 \\
98 & 381 \\
115 & 353 \\
20 & 154 \\
17 & 117 \\
246 & 297 \\
% Continue as needed...
\hline
\end{tabular}
\end{minipage}
\label{tab:identity_pairs}
\end{table}
